# Supplementary material for: Banshee: Bandwidth-Efficient DRAM Caching Via Software/Hardware Cooperation
Source: arXiv:1704.02677 source file (2017-04-10)
Supplement: Supplementary file 1 [file appendix.tex]

This paper was previously submitted to MICRO 2016. The major 
concern of multiple reviewers was that they wanted a more in-depth 
comparison to Tagless DRAM Cache (TDC). In particular, they asked
for a clear distinction
to be made between \name and that prior work because, similar to \name,
TDC also uses PTE/TLB for cache content tracking.  For this submission, we 
added considerable discussion about TDC throughout the paper and compared
\name to TDC both qualitatively and quantitatively. Specifically,
\name solves the 
address consistency and page aliasing problem in TDC (\cref{sec:pte}), 
simplifies the TLB coherence mechanism (\cref{sec:coherence}) and 
significantly improves the DRAM bandwidth efficiency for DRAM cache 
replacement (\cref{sec:fbr}).  For our modeled systems and workloads,
these differences lead to better performance and DRAM bandwidth efficiency
for \name, as we show quantitatively (\cref{sec:eval-main}).  This is despite
optimistic assumptions for TDC about TLB coherence overhead (TDC not charged
anything, but \name pays a cost), address consistency overhead (assumed to be
free for TDC, and none incurred for \name), and footprint cache (assumed to
be ideal for TDC, but not present for \name.

%We also addressed the following issues, amongst others.
%
%\begin{compactenum}
%
%\item We briefly analyze the hardware storage overhead of the tag 
%buffer and PTE/TLB extra bits in \name (\cref{sec:meth}).
%
%\item We emphasize why \texttt{lbm} has suboptimal performance for 
%\name in \cref{fig:speedup}, and point out how this can be 
%potentially solved using a hybrid FBR/LRU scheme.
%
%\item We emphasize that the reverse address mapping mechanism used by
%\name for migrating information from the tag buffer to the page table is
%not something \name introduces into the system --- modern operating systems 
%have such a mechanism already.
%
%\item We briefly explain how to implement LRU for tag buffer entries 
%that have the \textit{remap} bit cleared: we can use traditional LRU with 
%the \textit{remap} bits as a mask.
%
%\item We briefly discuss the tag buffer sensitivity in
%\cref{sec:eval-pt}.
%
%\item We explain that each experiment is run for 100 billion 
%instructions (\cref{sec:eval-bench}).
%
%\end{compactenum}
